# Supplementary material for: Inverse problem for a planar conductivity inclusion
Source: arXiv:2206.05593 source file (2023-01-19)
Supplement: Supplementary file 1 [file ex_supplement.pdf]

## SUPPLEMENTARY MATERIALS: An Example Article\*

Dianne Doe<sup>†</sup>, Paul T. Frank<sup>‡</sup>, and Jane E. Smith<sup>‡</sup>

**SM1. A detailed example.** Here we include some equations and theorem-like environments to show how these are labeled in a supplement and can be referenced from the main text. Consider the following equation:

$$(SM1.1) \quad a^2 + b^2 = c^2.$$

You can also reference equations such as (2.1) and (2.2b) from the main article in this supplement.

Vivamus vehicula leo a justo. Quisque nec augue. Morbi mauris wisi, aliquet vitae, dignissim eget, sollicitudin molestie, ligula. In dictum enim sit amet risus. Curabitur vitae velit eu diam rhoncus hendrerit. Vivamus ut elit. Praesent mattis ipsum quis turpis. Curabitur rhoncus neque eu dui. Etiam vitae magna. Nam ullamcorper. Praesent interdum bibendum magna. Quisque auctor aliquam dolor. Morbi eu lorem et est porttitor fermentum. Nunc egestas arcu at tortor varius viverra. Fusce eu nulla ut nulla interdum consectetur. Vestibulum gravida. Morbi mattis libero sed est.

Nam quis enim. Quisque ornare dui a tortor. Fusce consequat lacus pellentesque metus. Duis euismod. Duis non quam. Maecenas vitae dolor in ipsum auctor vehicula. Vivamus nec nibh eget wisi varius pulvinar. Cras a lacus. Etiam et massa. Donec in nisl sit amet dui imperdiet vestibulum. Duis porttitor nibh id eros.

### Theorem SM1.1. *An example theorem.*

Mauris consectetur, wisi eu lobortis scelerisque, urna nibh feugiat quam, id congue eros justo eget orci. Ut tellus. Maecenas mattis sapien sed eros. Aliquam quis lectus. Donec nec massa ac turpis semper cursus. Etiam consectetur ante vel odio. Aliquam tincidunt felis non dolor. Cras id augue ut nisl pretium placerat. Phasellus sapien sapien, pharetra sed, aliquam nec, suscipit a, nibh. Suspendisse risus. Nulla ut mi eget tellus sollicitudin euismod. Vestibulum malesuada malesuada dui. Ut at est ac dui aliquam sagittis. Aliquam erat volutpat.

### Lemma SM1.2. *An example lemma.*

Curabitur ullamcorper est in mauris. Praesent ac massa. Quisque enim odio, lobortis nec, mattis ut, luctus et, mauris. Mauris eu risus. Cum sociis natoque penatibus et magnis dis parturient montes, nascetur ridiculus mus. Duis eu ligula. Nulla vehicula leo tincidunt erat. Maecenas et nunc. Sed ut sapien. Vestibulum in est. Vestibulum rhoncus.

\*Submitted to the editors DATE.

**Funding:** This work was funded by the Fog Research Institute under contract no. FRI-454.

<sup>†</sup>Imagination Corp., Chicago, IL ([ddoe@imag.com](mailto:ddoe@imag.com), <http://www.imag.com/~ddoe/>).

<sup>‡</sup>Department of Applied Mathematics, Fictional University, Boise, ID ([ptfrank@fictional.edu](mailto:ptfrank@fictional.edu), [jesmith@fictional.edu](mailto:jesmith@fictional.edu)).

Donec metus metus, condimentum eu, accumsan nec, vulputate non, purus. Vestibulum ullamcorper vehicula sapien. Mauris risus odio, hendrerit ac, congue ac, ullamcorper at, odio. Aenean leo justo, commodo vitae, placerat blandit, malesuada vel, sem. Donec sit amet ante eget mauris adipiscing sollicitudin. Curabitur posuere sem et leo. Nulla ultricies mauris. Vestibulum ante ipsum primis in faucibus orci luctus et ultrices posuere cubilia Curae; Fusce sollicitudin augue vel tellus. Vivamus mauris eros, pharetra vel, lacinia pretium, egestas a, nibh. Morbi a ligula.

Donec vitae turpis. Suspendisse porttitor. Mauris aliquam purus vitae tellus. Morbi metus diam, tempus ac, cursus ut, ultricies quis, nulla. Praesent nec justo. In lobortis. Donec nec lectus a neque laoreet rhoncus. Quisque in risus nec wisi lacinia ullamcorper. In placerat. Proin facilisis sollicitudin libero. Integer eget neque et pede placerat aliquet. Aliquam purus nulla, pulvinar ut, facilisis quis, sodales sed, magna. Curabitur nulla lectus, rutrum id, bibendum ut, sagittis eget, diam. Sed porta dolor eget est. Integer hendrerit orci. In hac habitasse platea dictumst.

Here is an example citation: [SM1].

**SM2. Proof of Theorem 2.1.** Ut facilisis. Lorem ipsum dolor sit amet, consectetur adipiscing elit. Sed pellentesque, turpis sit amet aliquet porta, risus odio venenatis felis, at porta tellus lacus vitae nisl. Donec augue. Quisque consequat, pede laoreet pellentesque posuere, urna sapien tempor justo, eu aliquam tortor nunc id mauris. Fusce pretium, purus facilisis consequat mattis, ligula leo pretium mauris, ac suscipit augue sapien sit amet ipsum. Praesent et ligula eget tortor dapibus blandit. Duis rutrum felis eget dolor. Vestibulum quis elit. Integer dignissim, velit at scelerisque congue, ipsum nulla dignissim dolor, lacinia scelerisque neque erat a mi. Lorem ipsum dolor sit amet, consectetur adipiscing elit. Quisque ipsum lectus, euismod et, lacinia eu, iaculis eu, pede. Etiam justo quam, cursus ut, vulputate vel, feugiat ut, eros. Fusce eleifend mollis ipsum.

Nulla facilisi. Nunc nec elit. Integer ornare convallis tortor. Proin ac diam. In est sapien, laoreet euismod, mattis a, tincidunt at, risus. Vivamus risus. Vestibulum aliquam, urna aliquam porttitor accumsan, nulla tortor ullamcorper elit, ut consequat augue purus sit amet libero. Vivamus nisl lacus, commodo vel, dignissim ut, vestibulum id, pede. Curabitur malesuada hendrerit libero. Mauris quis dolor in tellus varius posuere. Sed vulputate elit at wisi. Fusce vitae neque. Nulla consectetur, nunc ac eleifend laoreet, mi nulla commodo wisi, vel faucibus ligula lectus ut arcu. Vivamus hendrerit.

Sed varius, nulla vitae tincidunt lobortis, nibh ipsum sollicitudin libero, et commodo tellus massa in neque. Nulla facilisi. Aenean nec lectus. Aliquam fermentum. Duis ut magna et augue interdum gravida. Morbi elit. Fusce malesuada tempus ipsum. Cum sociis natoque penatibus et magnis dis parturient montes, nascetur ridiculus mus. Mauris iaculis enim non metus. Nullam dui magna, congue et, suscipit sed, aliquam vel, turpis. Quisque ultricies.

Suspendisse feugiat sapien laoreet ante. Integer fringilla, erat eget adipiscing ultrices, nibh dui sollicitudin nunc, in lobortis arcu odio vitae erat. Fusce bibendum ultricies lacus. Mauris eleifend ligula a ante. Etiam faucibus cursus pede. Mauris enim eros, malesuada eu, mattis sit amet, blandit in, nulla. Fusce sit amet purus id mi posuere tincidunt. Mauris sit amet quam vitae quam semper accumsan. Lorem ipsum dolor sit amet, consectetur adipiscing elit. Nam a justo at quam accumsan euismod. Duis tincidunt tristique risus. Ut vel nibh

77 vel libero varius malesuada. In hac habitasse platea dictumst. Morbi sagittis mattis lorem.  
78 Pellentesque metus tellus, rutrum vitae, malesuada et, pharetra accumsan, ante. Quisque ac  
79 metus ac nisl gravida pellentesque. Sed dapibus feugiat sapien. Vestibulum nec nunc eget  
80 sem aliquam lobortis. Suspendisse aliquam quam quis metus.

81 Suspendisse in odio. In elit diam, cursus vitae, venenatis in, molestie in, leo. Cras ornare.  
82 Nulla libero. Phasellus feugiat mattis libero. Sed vehicula aliquam ligula. Nullam lacinia,  
83 felis vel dignissim sodales, enim lectus lobortis diam, quis nonummy mauris odio auctor tortor.  
84 Integer in dui nec lacus bibendum ultrices. Etiam odio elit, aliquam et, porttitor id, interdum  
85 cursus, elit. Nulla eleifend tempor mauris. In vel arcu quis pede laoreet vulputate.

86 Morbi pharetra magna a lorem. Cras sapien. Duis porttitor vehicula urna. Phasellus  
87 iaculis, mi vitae varius consequat, purus nibh sollicitudin mauris, quis aliquam felis dolor vel  
88 elit. Quisque neque mi, bibendum non, tristique convallis, congue eu, quam. Etiam vel felis.  
89 Quisque ac ligula at orci pulvinar rutrum. Donec mi eros, sagittis eu, consectetur sed, sagittis  
90 sed, lorem. Nunc sed eros. Nullam pellentesque ante quis lectus. Vivamus lacinia, sapien vel  
91 fermentum placerat, purus nisl aliquet odio, et porta wisi dui nec nunc. Fusce porta cursus  
92 libero.

93 Quisque eu mi a augue mollis posuere. Donec tincidunt, lorem at vestibulum pulvinar,  
94 felis purus nonummy urna, at accumsan purus dui nec leo. Praesent tortor turpis, vehicula in,  
95 aliquet ut, dignissim ac, leo. Curabitur sagittis mi id eros. In magna. Sed vitae elit facilisis  
96 elit semper sollicitudin. Curabitur convallis tempor nulla. Nullam non turpis a pede sagittis  
97 ultrices. Etiam vulputate pede in ligula. Sed a ante id metus pellentesque suscipit. Sed  
98 adipiscing justo vitae sapien. Nunc posuere, pede ullamcorper gravida egestas, justo libero  
99 tincidunt arcu, vitae pellentesque arcu leo ut mauris. Pellentesque auctor mauris sit amet  
100 elit luctus fringilla. Cras sed wisi. Morbi luctus enim vitae tellus. Vivamus venenatis sodales  
101 libero.

102 **SM3. Additional experimental results.** Table 1 shows additional supporting evidence.

Table SM1

Example table.

| Species | Mean | Std. Dev. |
|---------|------|-----------|
| 1       | 3.4  | 1.2       |
| 2       | 5.4  | 0.6       |

REFERENCES

- 104 [1] T. G. KOLDA AND J. R. MAYO, *An adaptive shifted power method for computing generalized tensor*  
105 *eigenpairs*, SIAM Journal on Matrix Analysis and Applications, 35 (2014), pp. 1563–1581, <https://doi.org/10.1137/140951758>.  
106
